# Supplementary material for: Using Interventions to Improve Out-of-Distribution Generalization of Text-Matching Recommendation Systems
Source: arXiv:2210.10636 source file (2023-06-14)
Supplement: Supplementary file 1 [file appendix_main.tex]

\appendix

\section{Appendix}

Optionally include extra information (complete proofs, additional experiments and plots) in the appendix.
This section will often be part of the supplemental material.

\subsection{Proofs}
\subsection{Experimental Details}

\subsection{Presence of Attribute Labels in Datasets [In Progress]} 

From Causal shortcut removal: Such labels often appear in the form of metadata associated with training data—for example, labels of the background—but
are often not available at test time.
Auxiliary label: Typically available at training time (and assume not available at test time)\todo{add to main paper} -> \textbf{we make same assumption}

The presence of different kinds of distribution shifts in DG literature...
e.g., in Rotated MNIST \textit{domain} and \textit{attribute} (angle) point to similar entities whereas in Colored MNIST they do not. We have attempted to bridge the gap between different communities and propose a generalization by considering domain as one of the attributes

In fact, \cite{Koh2021WILDSAB} create different domains in WILDS using metadata of attribute
\begin{itemize}
    \item Often have labels by virtue of data collection 
\end{itemize}

\begin{table}[h!]
  \caption{Commonly used DG datasets and available attribute labels}
  \label{table:dataset_attrs}
  \centering
  \begin{tabular}{lcl}
    \toprule
%     \multicolumn{2}{c}{Part}                   \\
%     \cmidrule(r){1-2}
    \textbf{Dataset}     & \textbf{\#attributes provided} & \textbf{Attributes}  \\
    \midrule
    Waterbirds & 1 & Background (land/water) \\
    CelebA & 40 & Eyeglasses, Hair Color, Pointy Nose, Wearing Hat etc. \\
    FMoW (WILDS) & 2 & Time, Region \\
    CivilComments(WILDS) & 8 & Demographic (male, female, LGBTQ, Christian,\\
    & & Muslim, other religions, Black, White)\\
    \bottomrule
  \end{tabular}
\end{table}
