# Supplementary material for: Using Interventions to Improve Out-of-Distribution Generalization of Text-Matching Recommendation Systems
Source: arXiv:2210.10636 source file (2023-06-14)
Supplement: Supplementary file 2 [file appendix_relatedwork.tex]

Papers on sentence matching:

- https://arxiv.org/pdf/1702.03814.pdf%E3%80%82Bilateral : Bilateral Multi-Perspective Matching for Natural Language Sentences
This paper starts with a nice list of scenarios for sentence matching

- https://proceedings.neurips.cc/paper/2014/file/b9d487a30398d42ecff55c228ed5652b-Paper.pdf: Convolutional Neural Network Architectures for
Matching Natural Language Sentences : Neurips 2014

- https://par.nsf.gov/servlets/purl/10233607 : Interactive Attention Networks for Semantic
Text Matching

- https://arxiv.org/pdf/2010.03099.pdf : DiPair: Fast and Accurate Distillation for Trillion-Scale
Text Matching and Pair Modeling

- https://arxiv.org/pdf/2010.08240.pdf : Augmented SBERT: Data Augmentation Method for Improving
Bi-Encoders for Pairwise Sentence Scoring Tasks

Papers on OOD in sentence-level tasks (not necessarily sentence matching):

- https://aclanthology.org/D18-1077.pdf: Out-of-domain Detection based on Generative Adversarial Network

- https://arxiv.org/pdf/2004.06100.pdf: Pretrained Transformers Improve Out-of-Distribution Robustness

- https://arxiv.org/pdf/2109.02431.pdf : On Length Divergence Bias in Textual Matching Models

- https://arxiv.org/pdf/1903.10794.pdf : RecSys-DAN: Discriminative Adversarial Networks
for Cross-Domain Recommender Systems

- https://arxiv.org/pdf/2106.00149.pdf : HiddenCut: Simple Data Augmentation for Natural Language
Understanding with Better Generalization

Other domain generalization papers:

- https://arxiv.org/pdf/2104.09937.pdf?ref=https://githubhelp.com: Gradient Matching for Domain Generalization

- https://arxiv.org/pdf/1907.04347.pdf : Cross-Domain Generalization of Neural Constituency Parsers

- https://proceedings.neurips.cc/paper/2018/file/647bba344396e7c8170902bcf2e15551-Paper.pdf : MetaReg: Towards Domain Generalization using
Meta-Regularization

- https://arxiv.org/pdf/1908.10763.pdf : Unlearn Dataset Bias in Natural Language Inference by Fitting the
Residual

- https://aclanthology.org/2020.emnlp-main.265/?ref=https://githubhelp.com : Learning to Contrast the Counterfactual Samples for Robust Visual Question Answering

- https://openreview.net/pdf?id=H1VGkIxRZ : ENHANCING THE RELIABILITY OF
OUT-OF-DISTRIBUTION IMAGE DETECTION IN
NEURAL NETWORKS : ICLR 2018

- https://proceedings.neurips.cc/paper/2018/file/2151b4c76b4dcb048d06a5c32942b6f6-Paper.pdf : Out-of-Distribution Detection using Multiple
Semantic Label Representations : NeurIPS 2018

- https://proceedings.mlr.press/v163/adila22a/adila22a.pdf : https://proceedings.mlr.press/v163/adila22a/adila22a.pdf : NeurIPS workshop 2021

- https://aclanthology.org/2021.emnlp-main.84/ : Contrastive Out-of-Distribution Detection for Pretrained Transformers : EMNLP 2021

- https://aclanthology.org/2021.emnlp-main.835/ : Types of Out-of-Distribution Texts and How to Detect Them : EMNLP 2021

a survey on domain generalization: https://arxiv.org/abs/2103.03097
