# Supplementary material for: Using Interventions to Improve Out-of-Distribution Generalization of Text-Matching Recommendation Systems
Source: arXiv:2210.10636 source file (2023-06-14)
Supplement: Supplementary file 3 [file exp_details.tex]

\subsection{Experimental Details}
